# Supplementary material for: Exploration of the High Entropy Alloy Space as a Constraint Satisfaction Problem
Source: arXiv:1712.02442 source file (2018-02-25)
Supplement: Supplementary file 1 [file Supplementary_Material.pdf]

# APPENDIX

## A. Thermo-Calc graphs

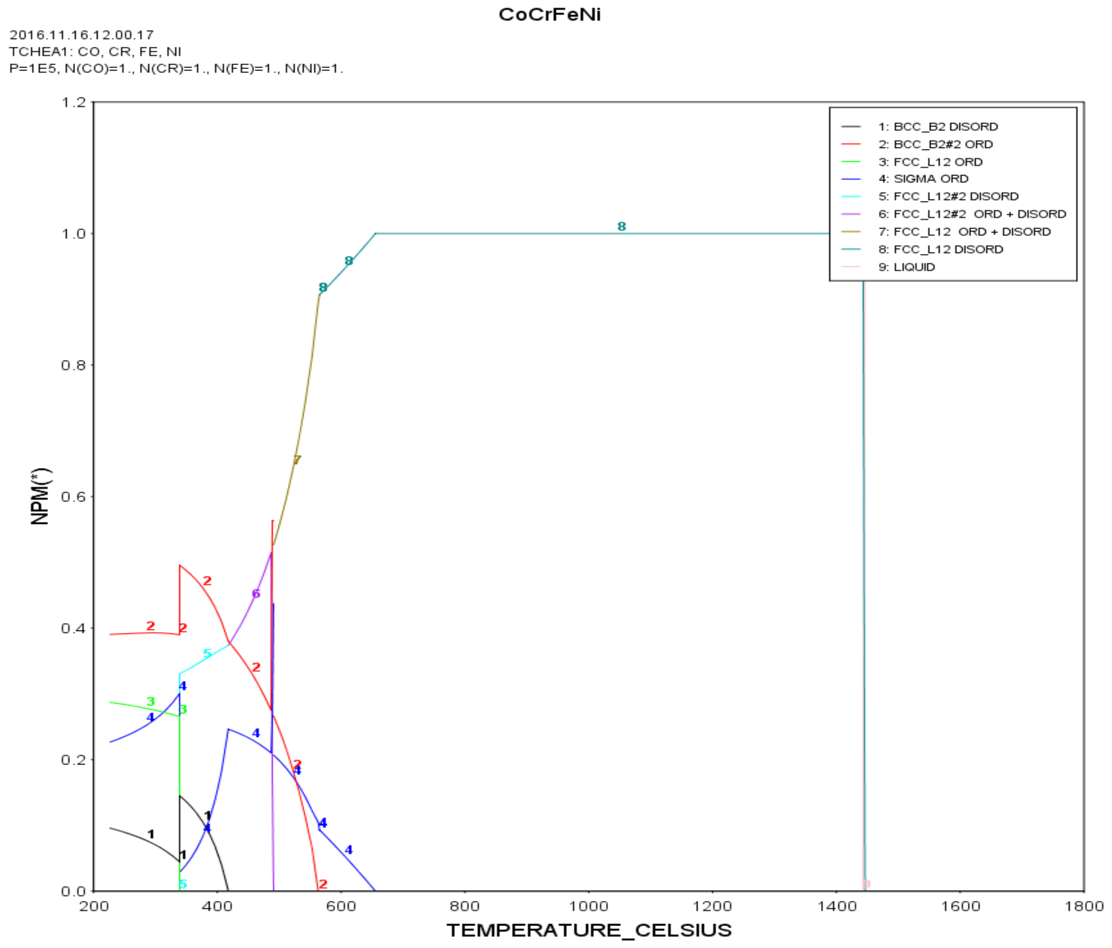


**Figure A1. Phase stability graph output from Thermo-Calc software**

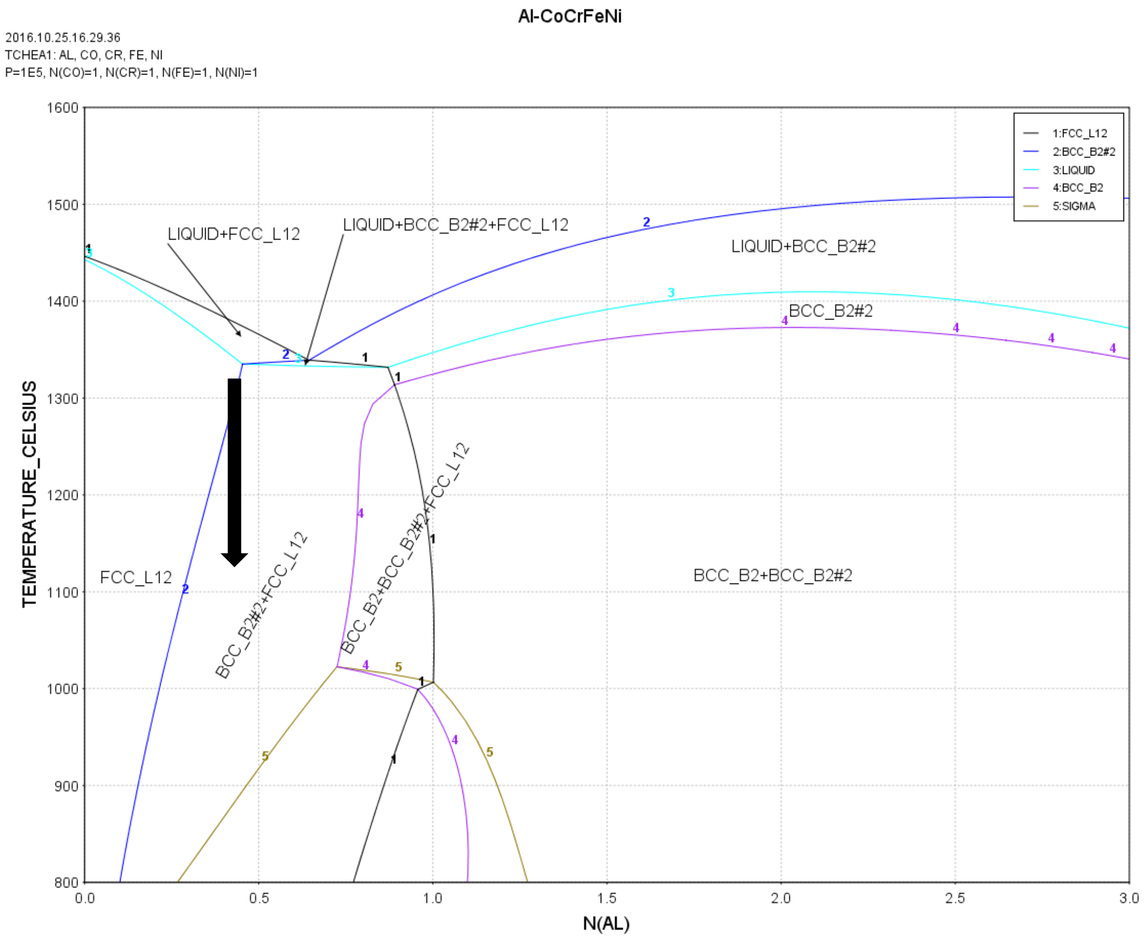


**Figure A2. AlCoCrFeNi isopleth showing a two-phase region under a single-phase solid solution region**

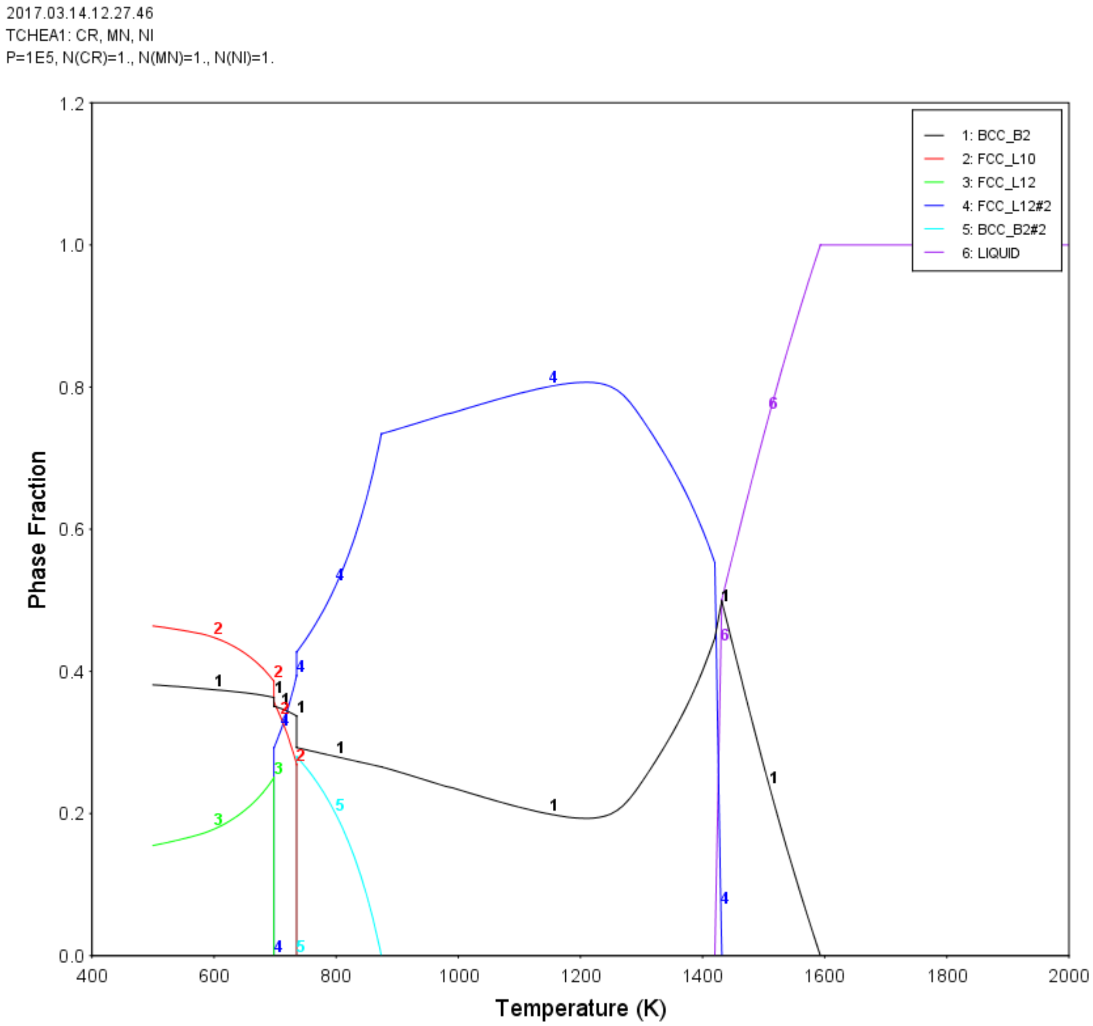


**Figure A3. Phase fraction graph of CrMnNi at an equiatomic concentration**

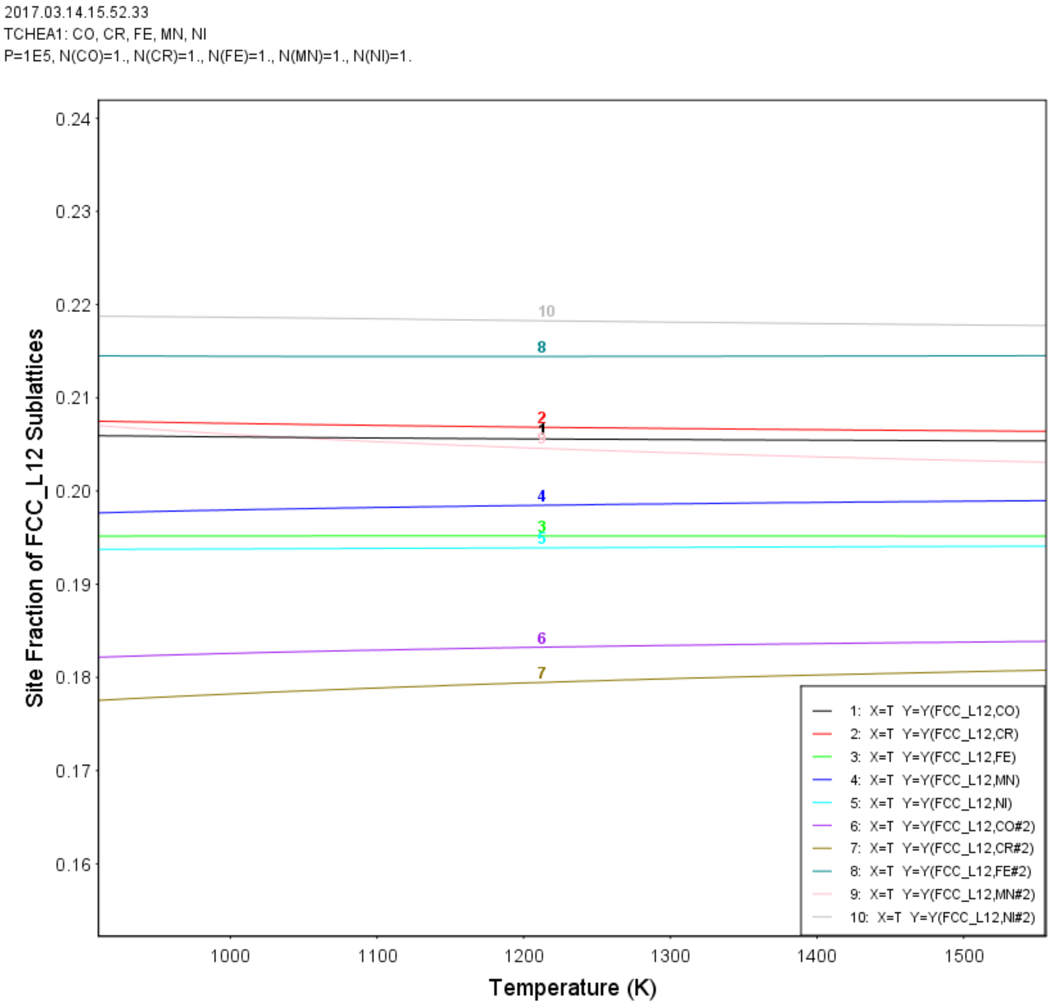


**Figure A4. Site fractions of FCC_L12 sublattices in CoCrFeMnNi between 1000-1500 K**

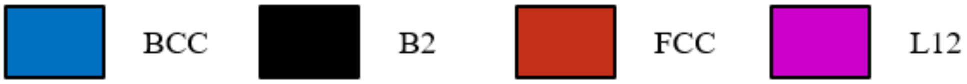


**Legend for Sections B, C, and D**

## B. Ternary visualizations

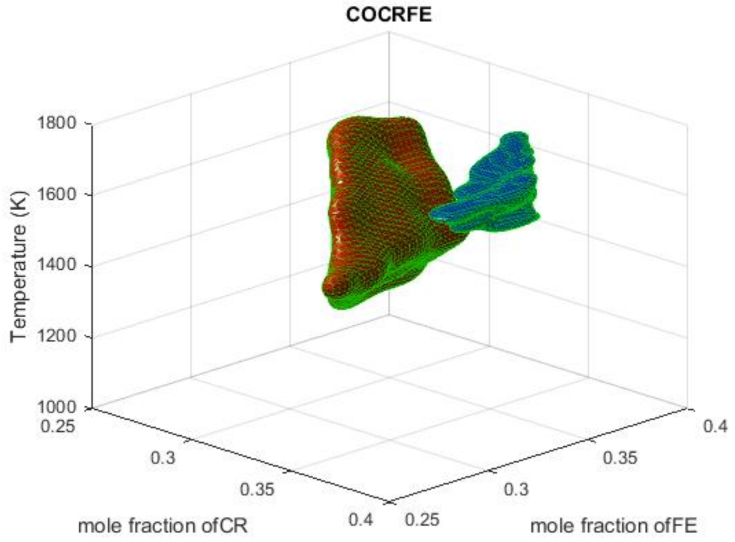


**Figure B1. Single-phase region visualization for CoCrFe**

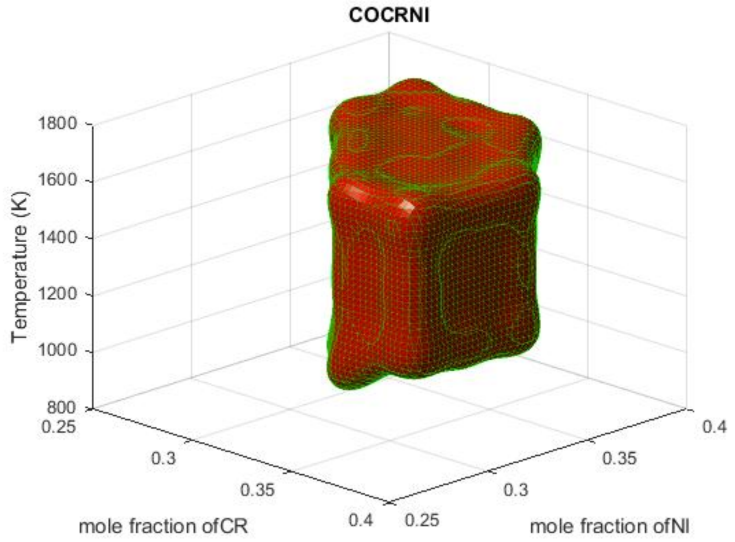


**Figure B2. Single-phase region visualization for CoCrNi**

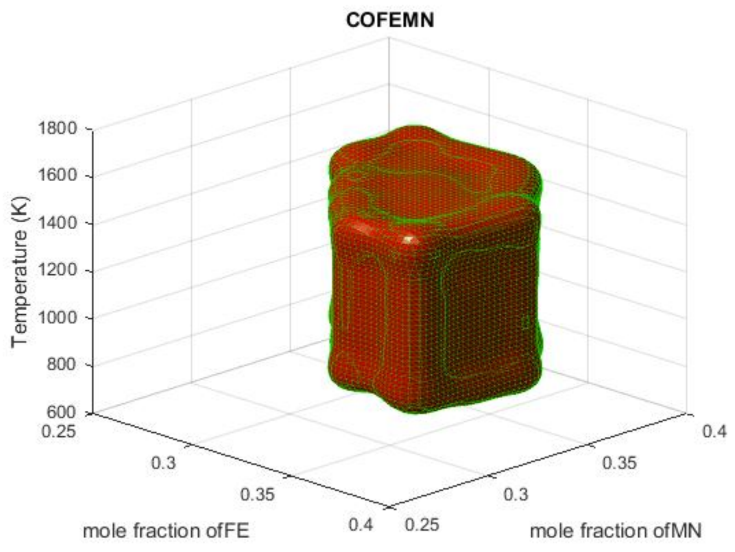


**Figure B3. Single-phase region visualization for CoFeMn**

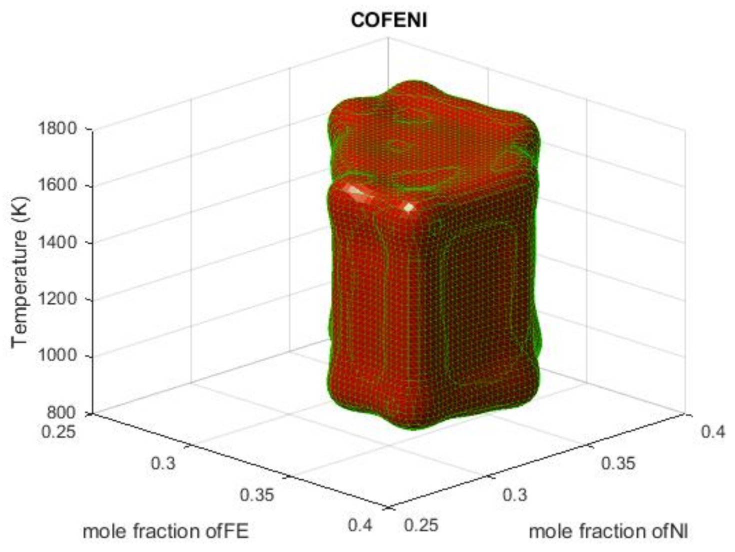


**Figure B4. Single-phase region visualization for CoFeNi**

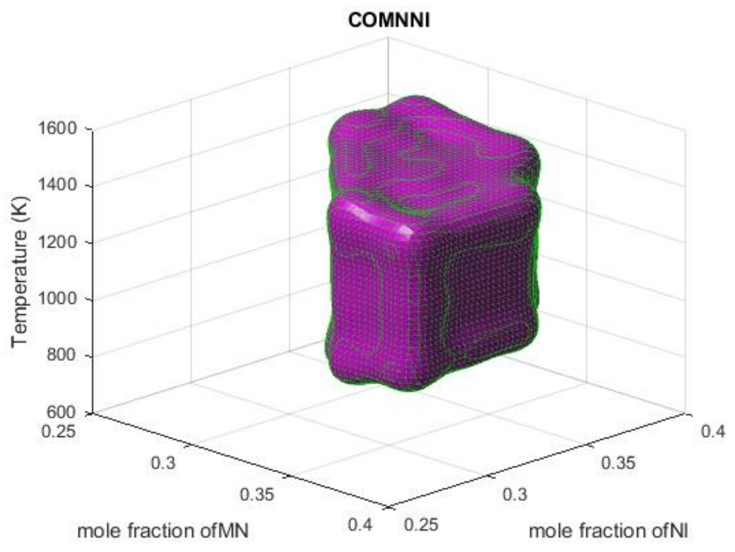


**Figure B5. Single-phase region visualization for CoMnNi**

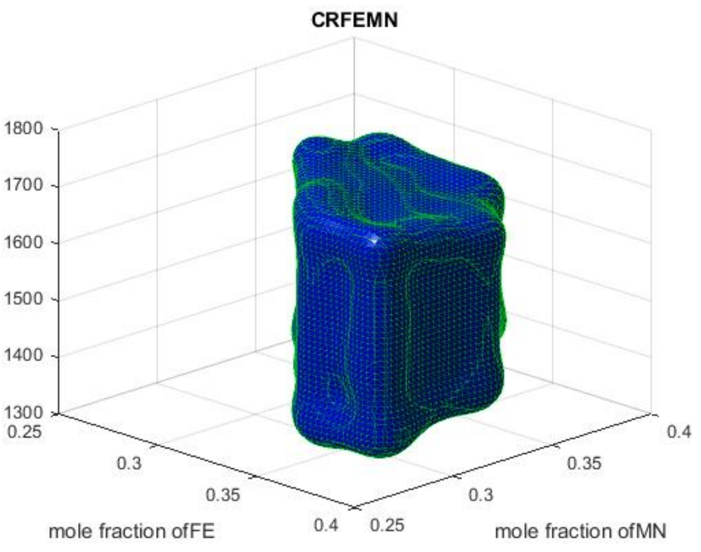


**Figure B6. Single-phase region visualization for CrFeMn**

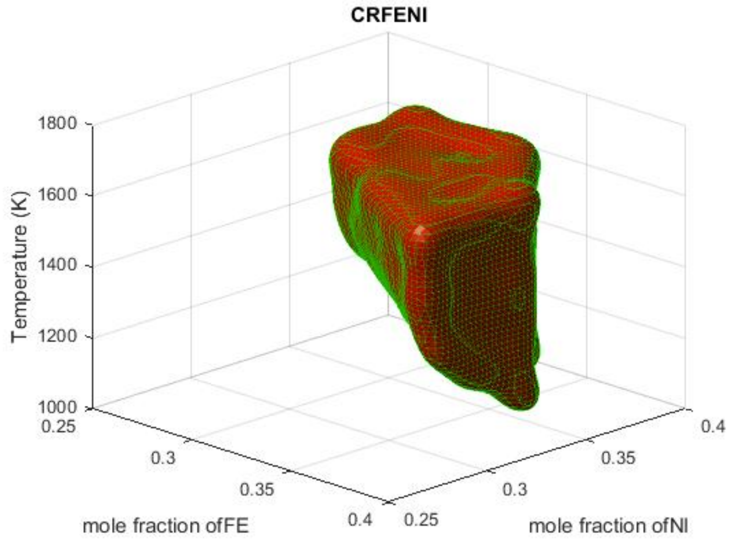


**Figure B7. Single-phase region visualization for CrFeNi**

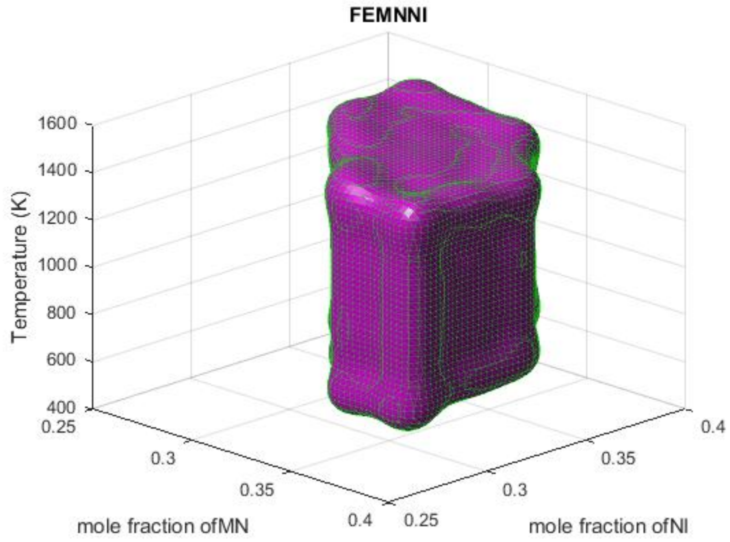


**Figure B8. Single-phase region visualization for FeMnNi**

## C. Quaternary visualizations

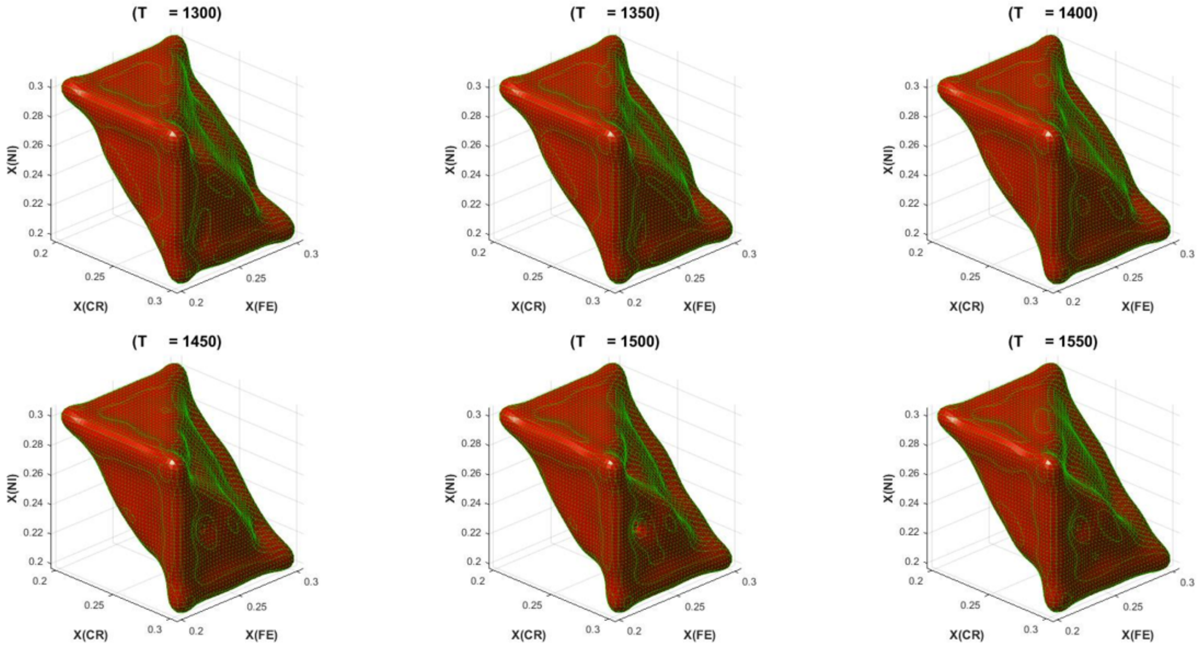


**Figure C1. Single-phase region visualizations for selected temperatures in CoCrFeNi**

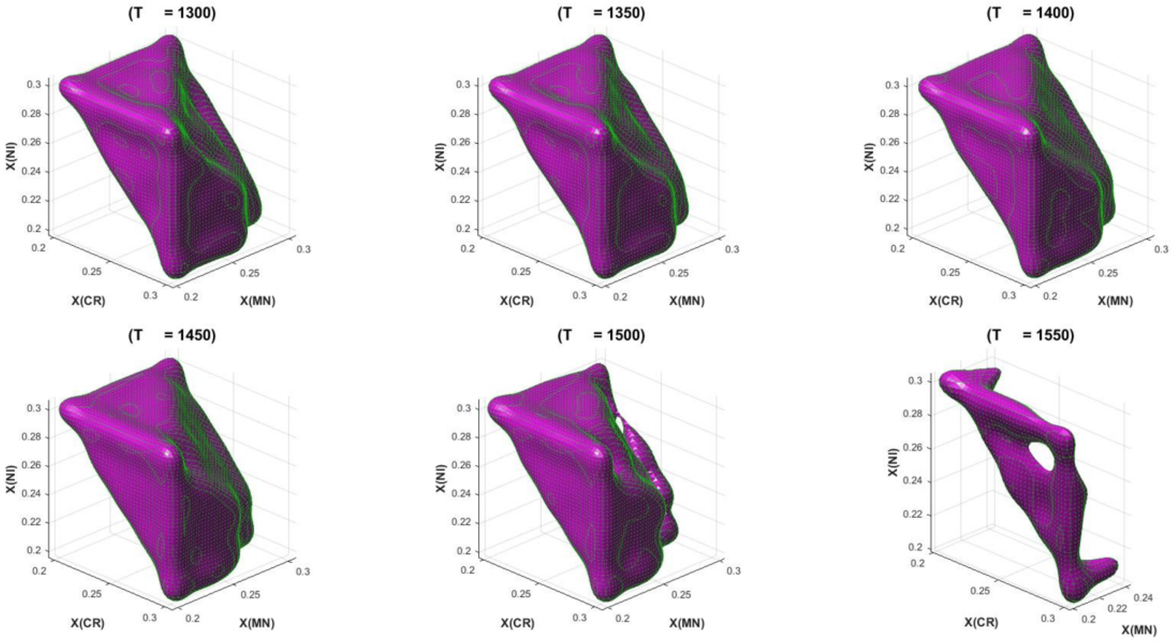


**Figure C2. Single-phase region visualizations for selected temperatures in CoCrMnNi**

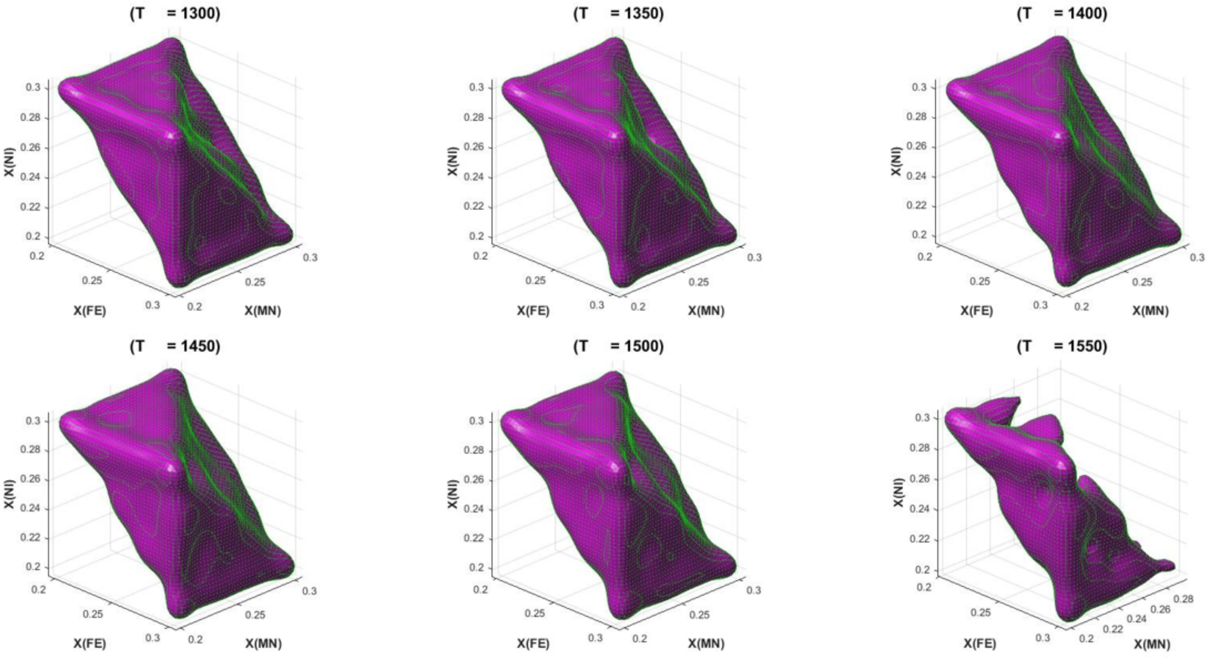


**Figure C3. Single-phase region visualizations for selected temperatures in CoFeMnNi**

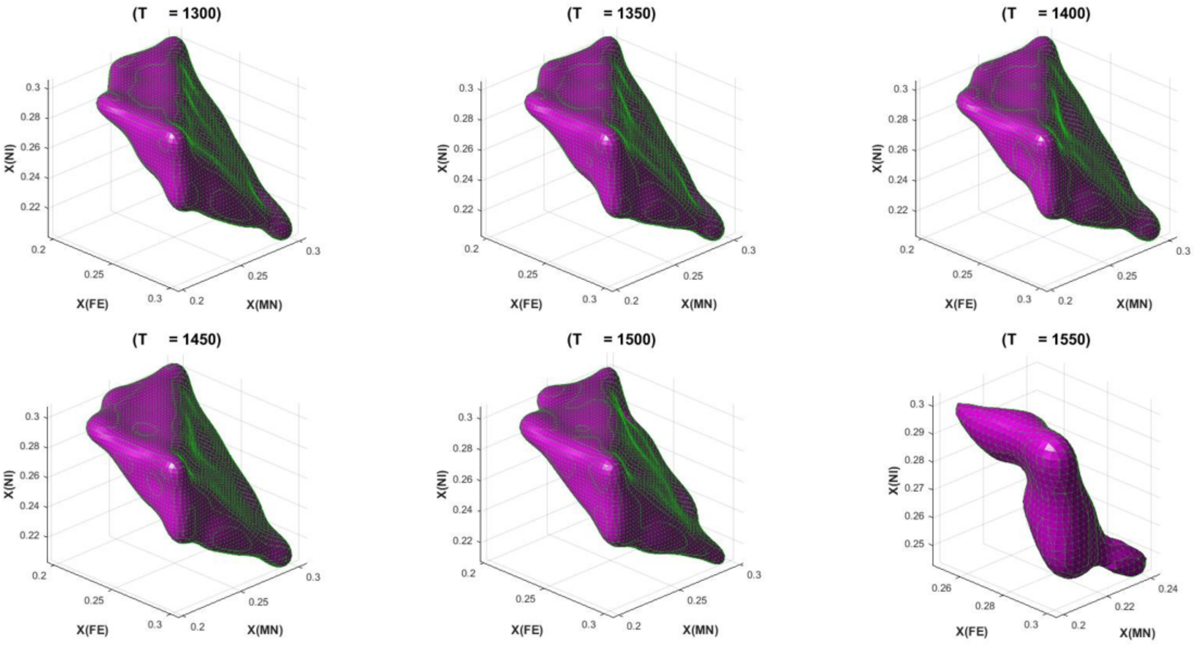


**Figure C4. Single-phase region visualizations for selected temperatures in CrFeMnNi**

## D. Precipitation hardening (AlCoCrFeNi)

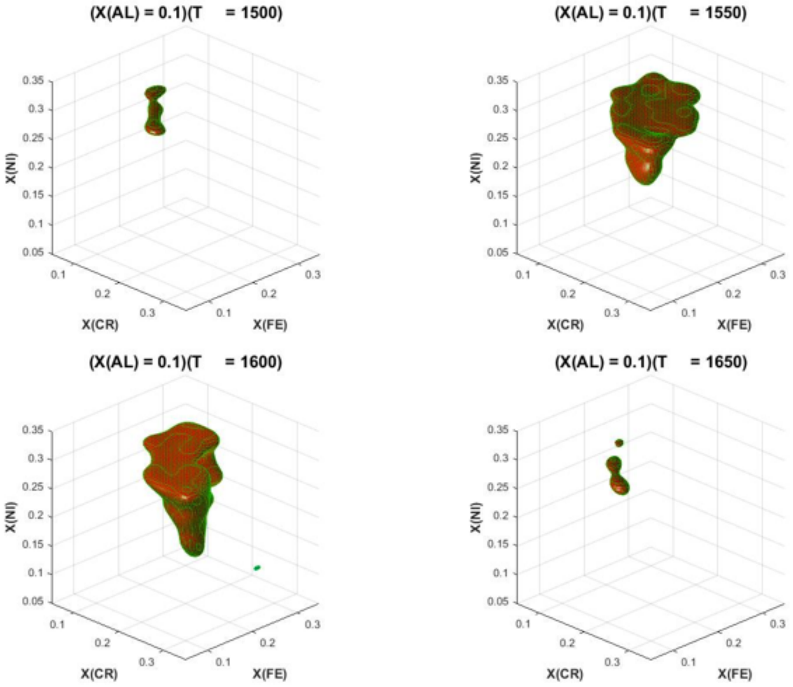


**Figure D1. Regions of precipitation hardenability with 10% atomic concentration of Al**

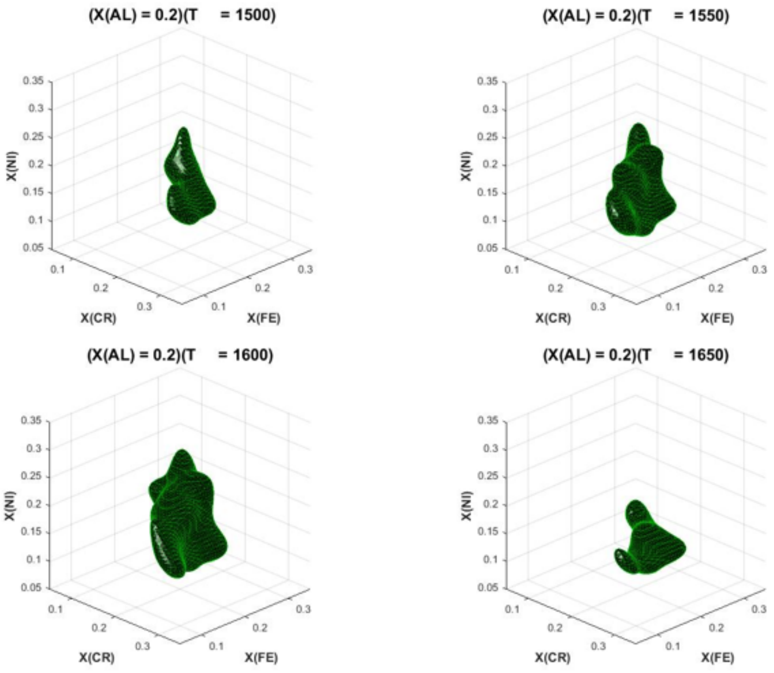


**Figure D2. Regions of precipitation hardenability with 20% atomic concentration of Al**

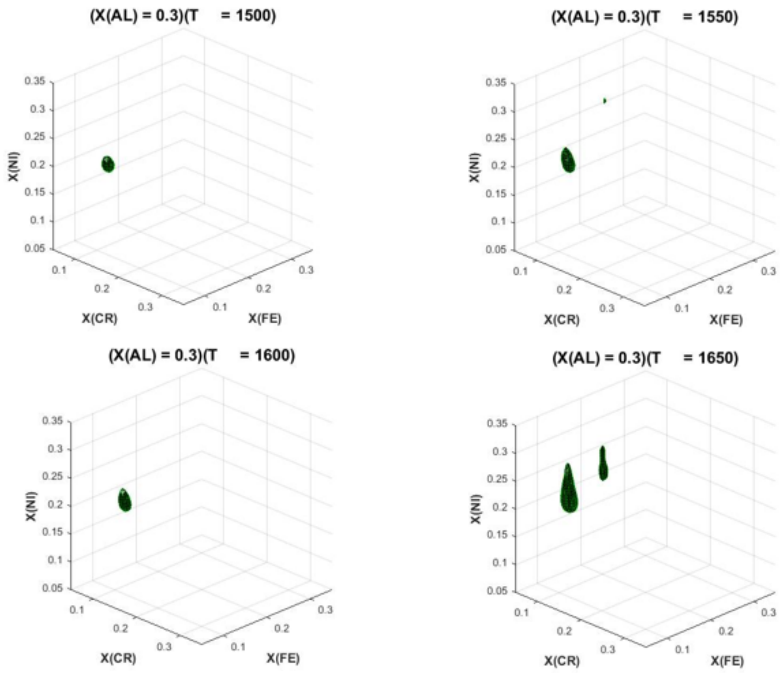


**Figure D3. Regions of precipitation hardenability with 30% atomic concentration of Al**

E. Verification

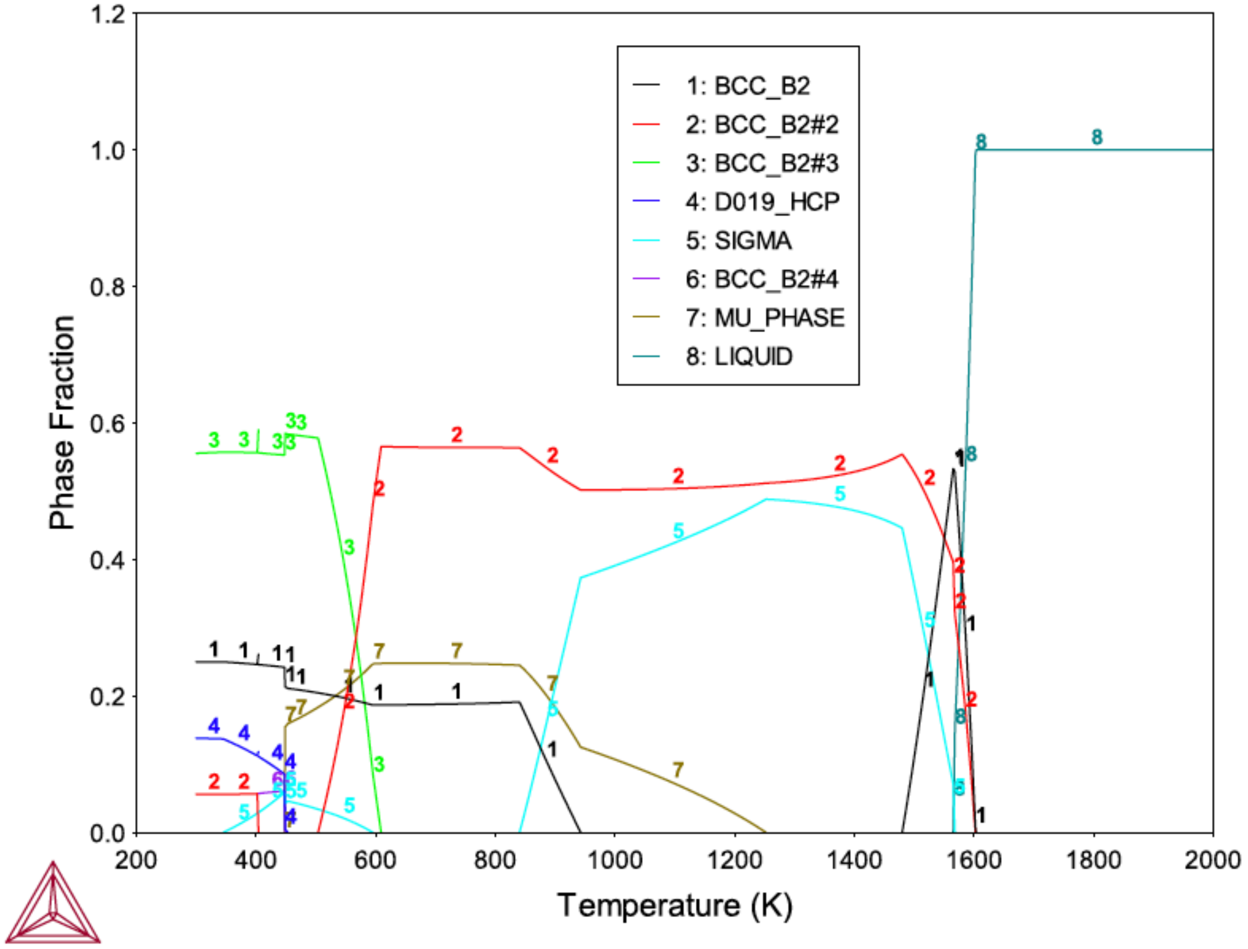


Figure E1. Phase fraction calculation in the $AlCoCr_{1.5}FeMo_{0.5}Ni$

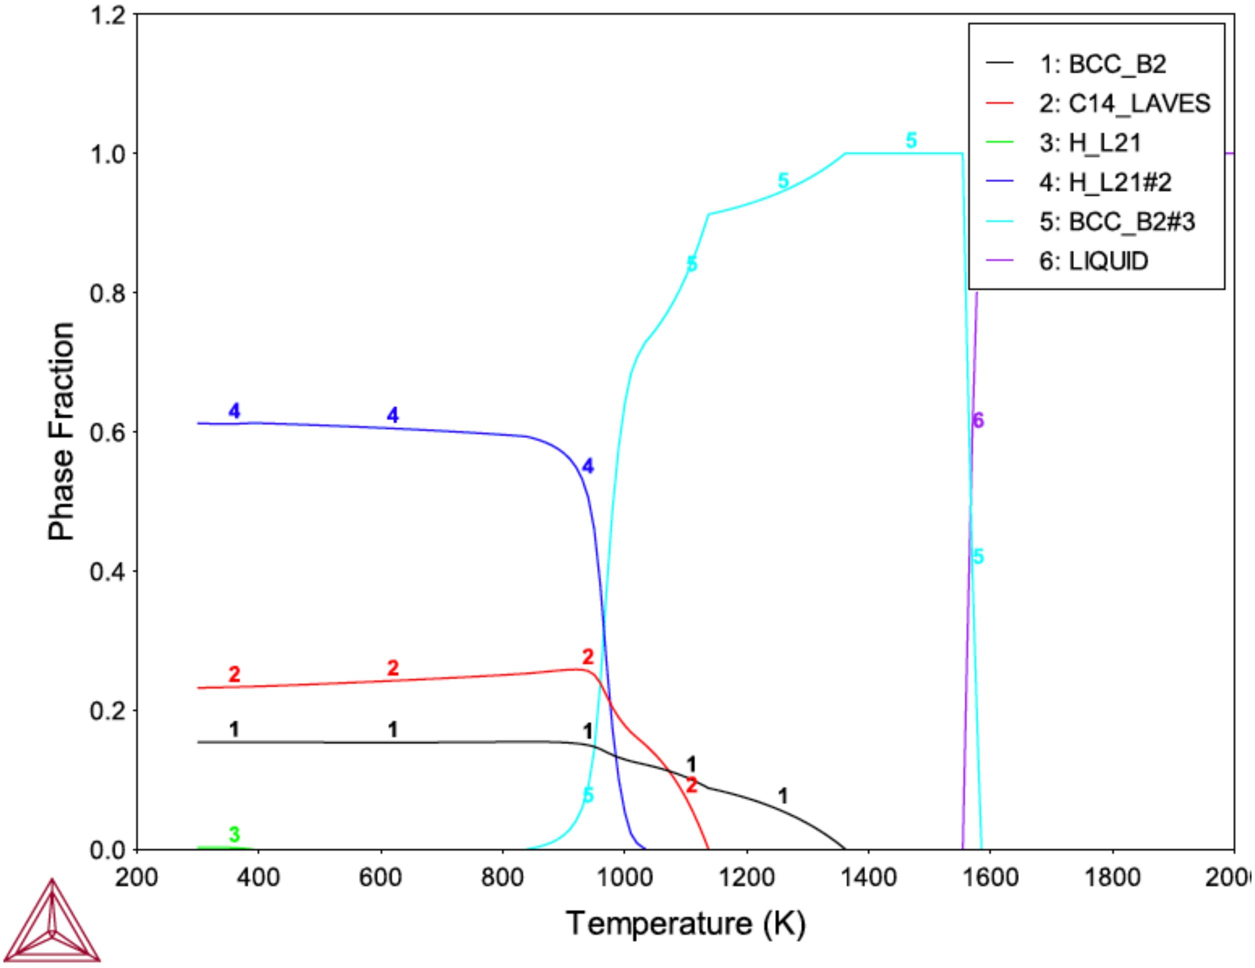


Figure E2. Phase fraction calculation in the AlCoCrFeNiTi

## F. Site-Fractions

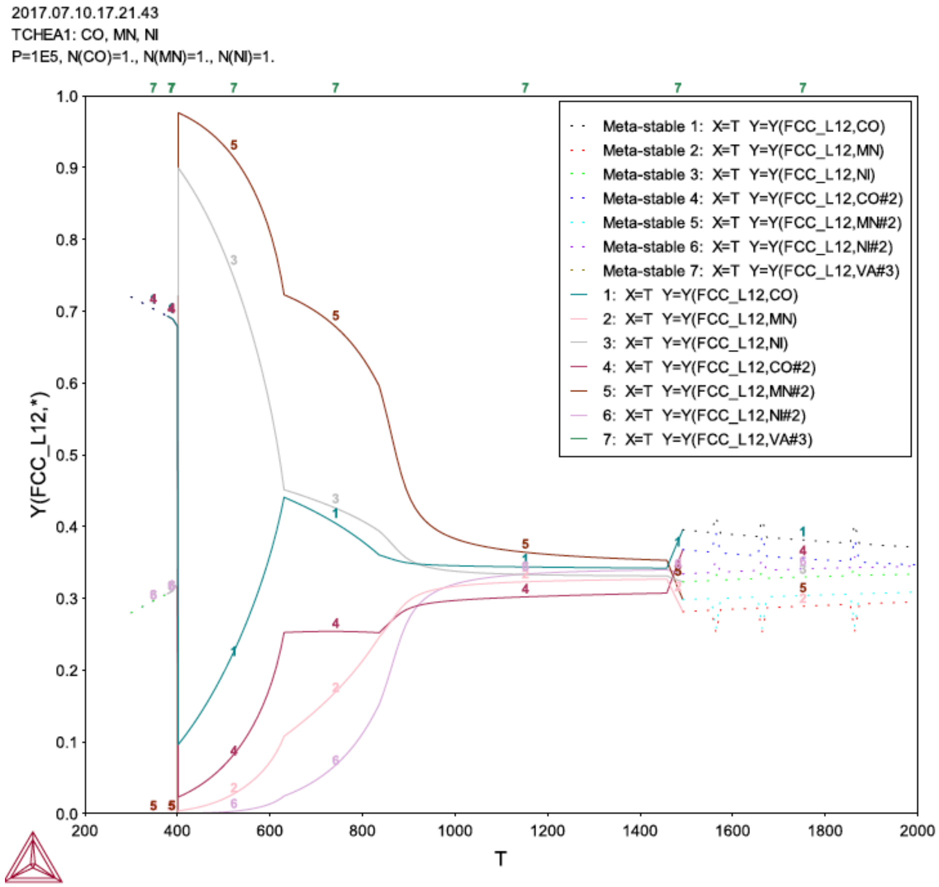


Figure F1. Site fraction calculations in the CoMnNi Ternary

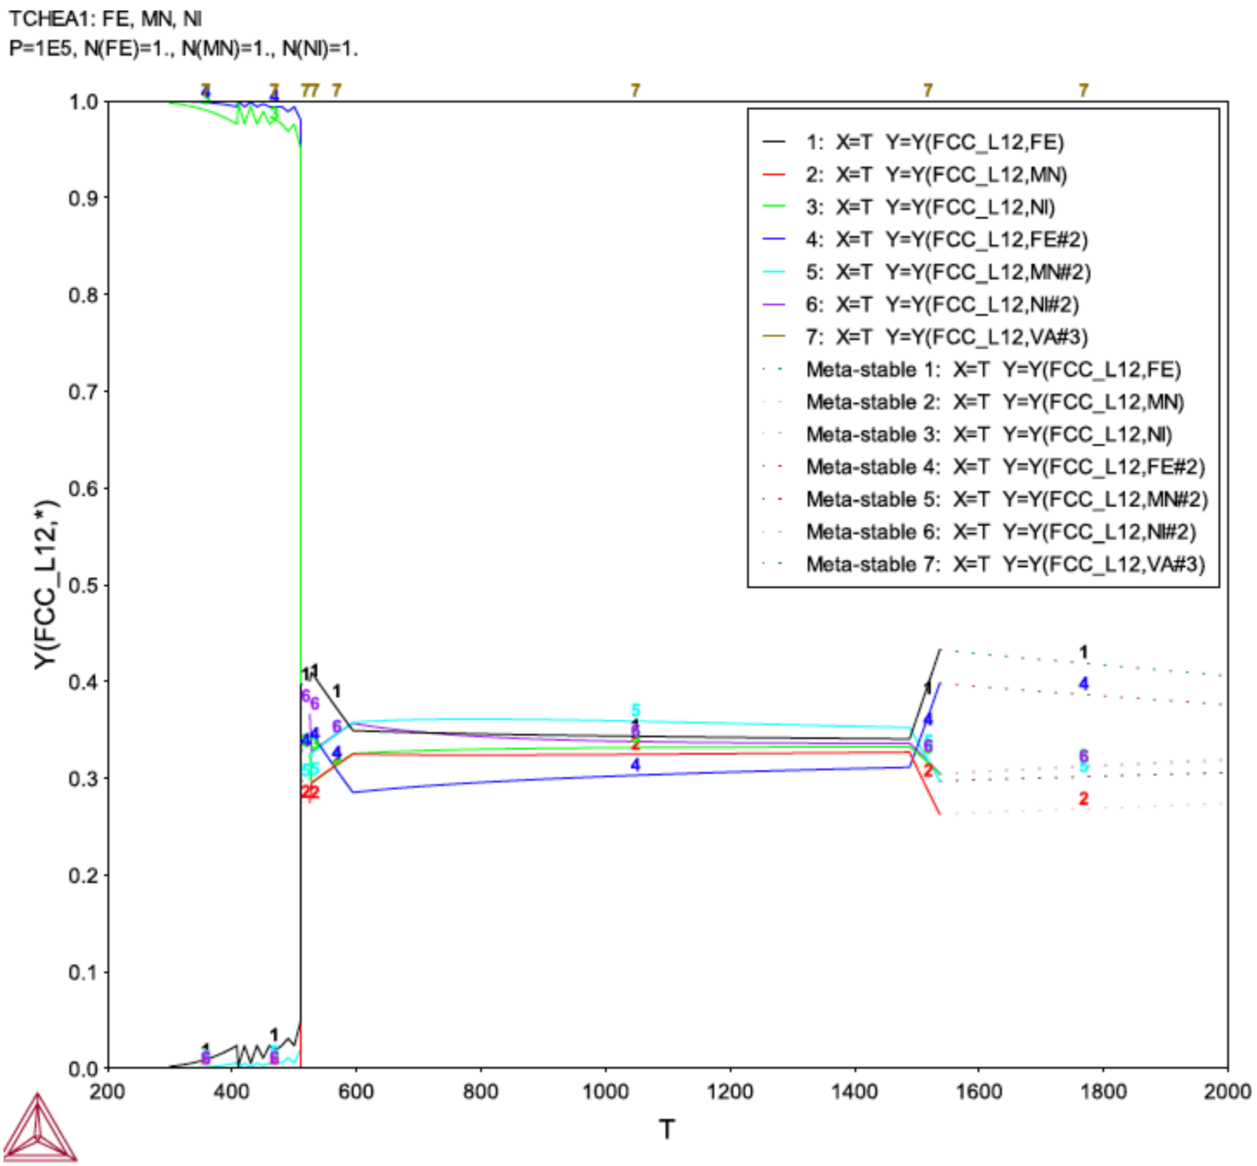


Figure F2. Site fraction calculations in the FeMnNi Ternary

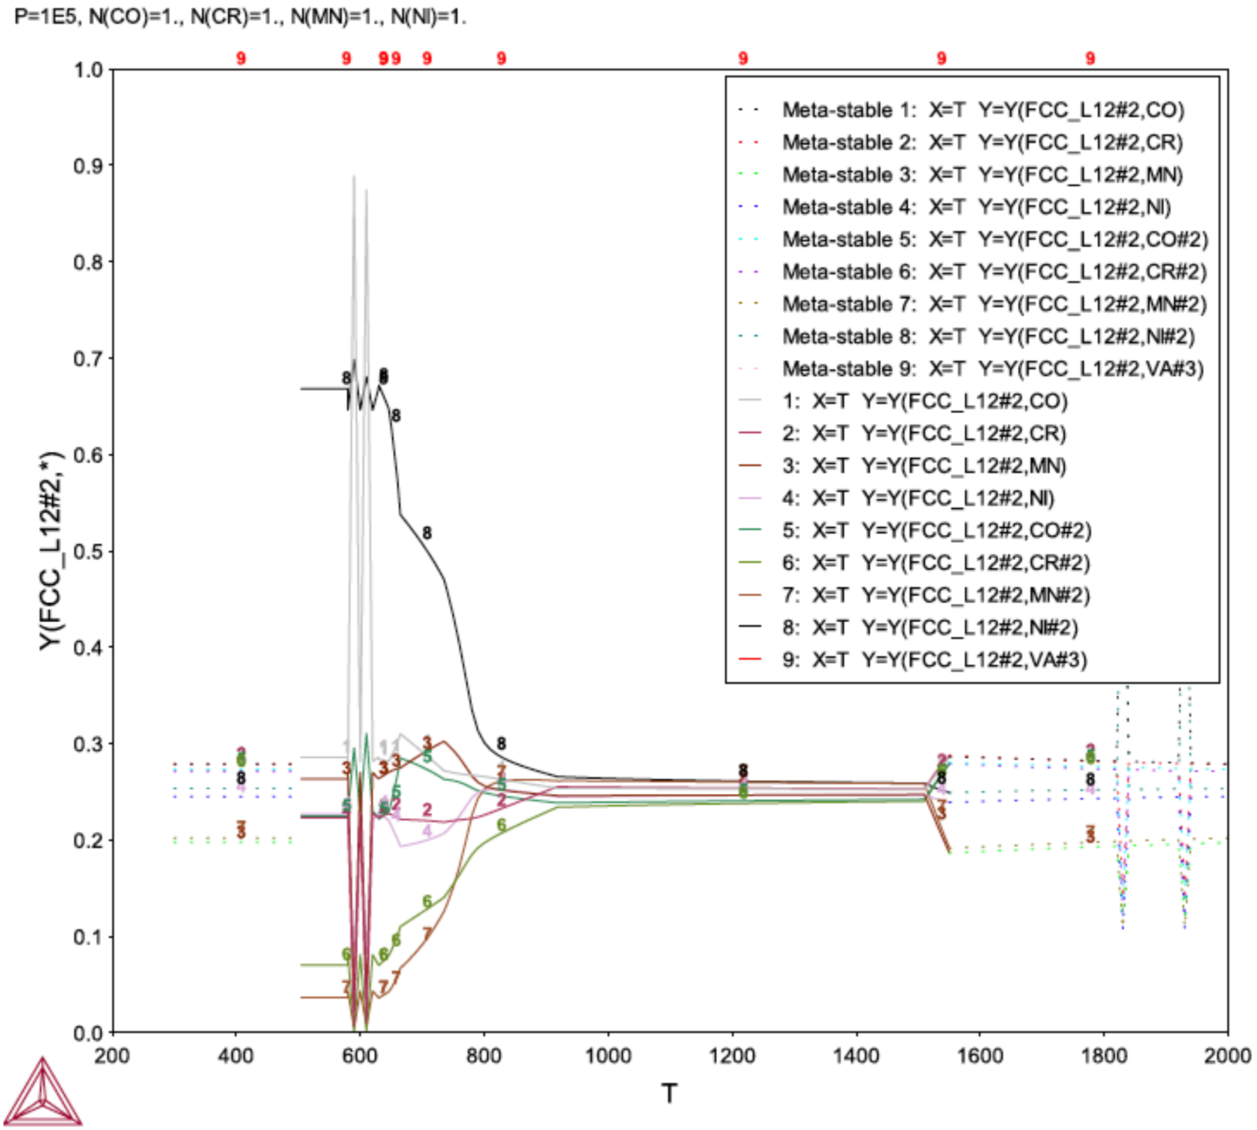


Figure F3. Site fraction calculations in the CoCrMnNi quaternary

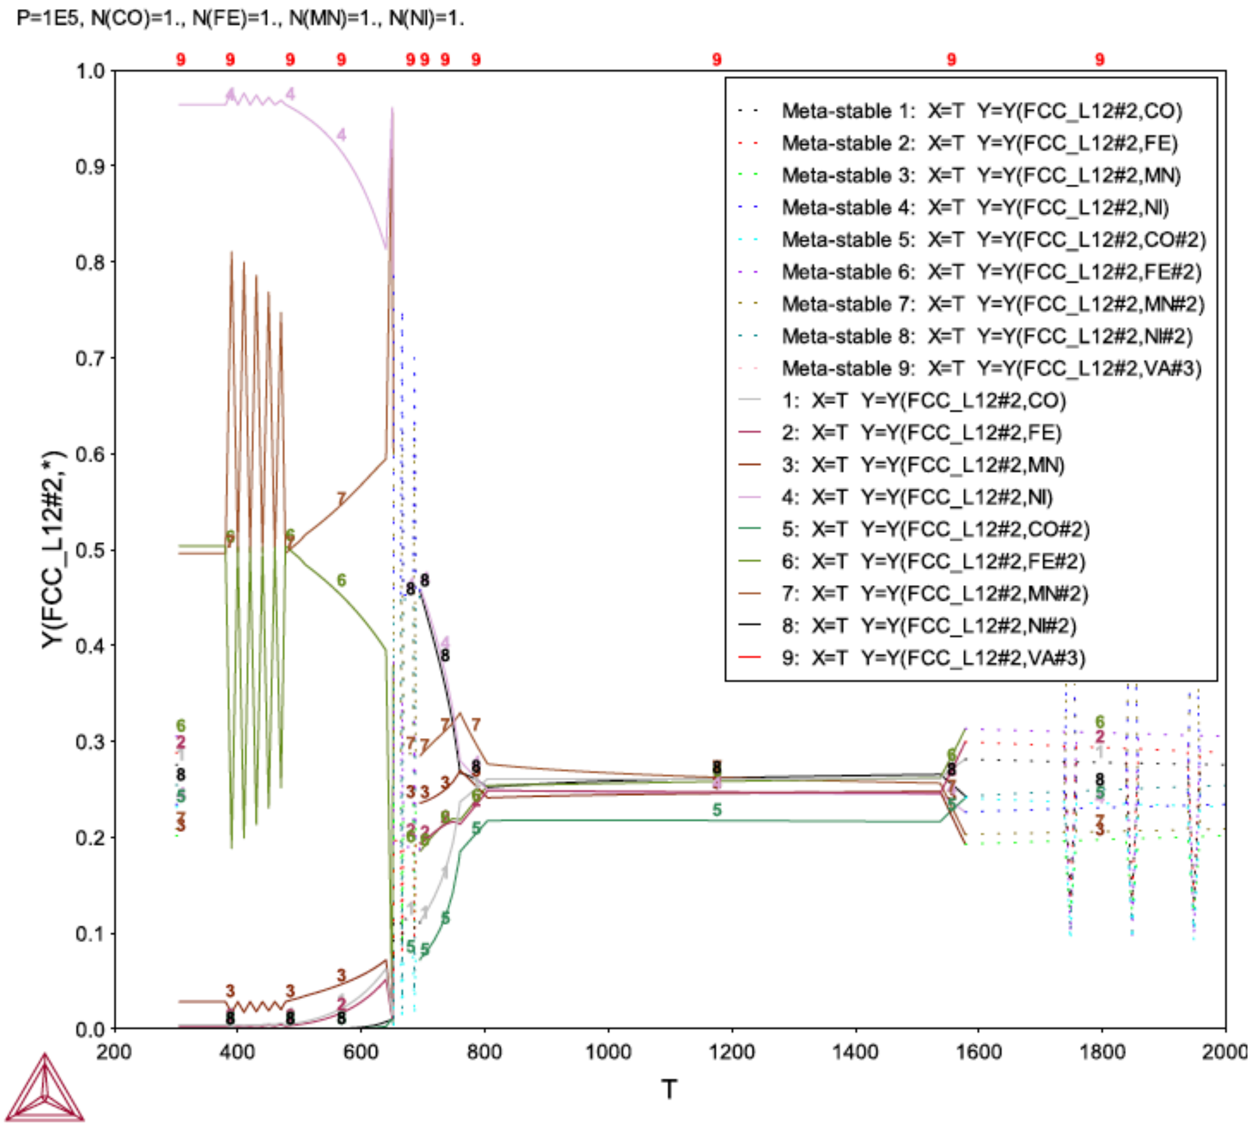


Figure F4. Site fraction calculations in the CoFeMnNi quaternary

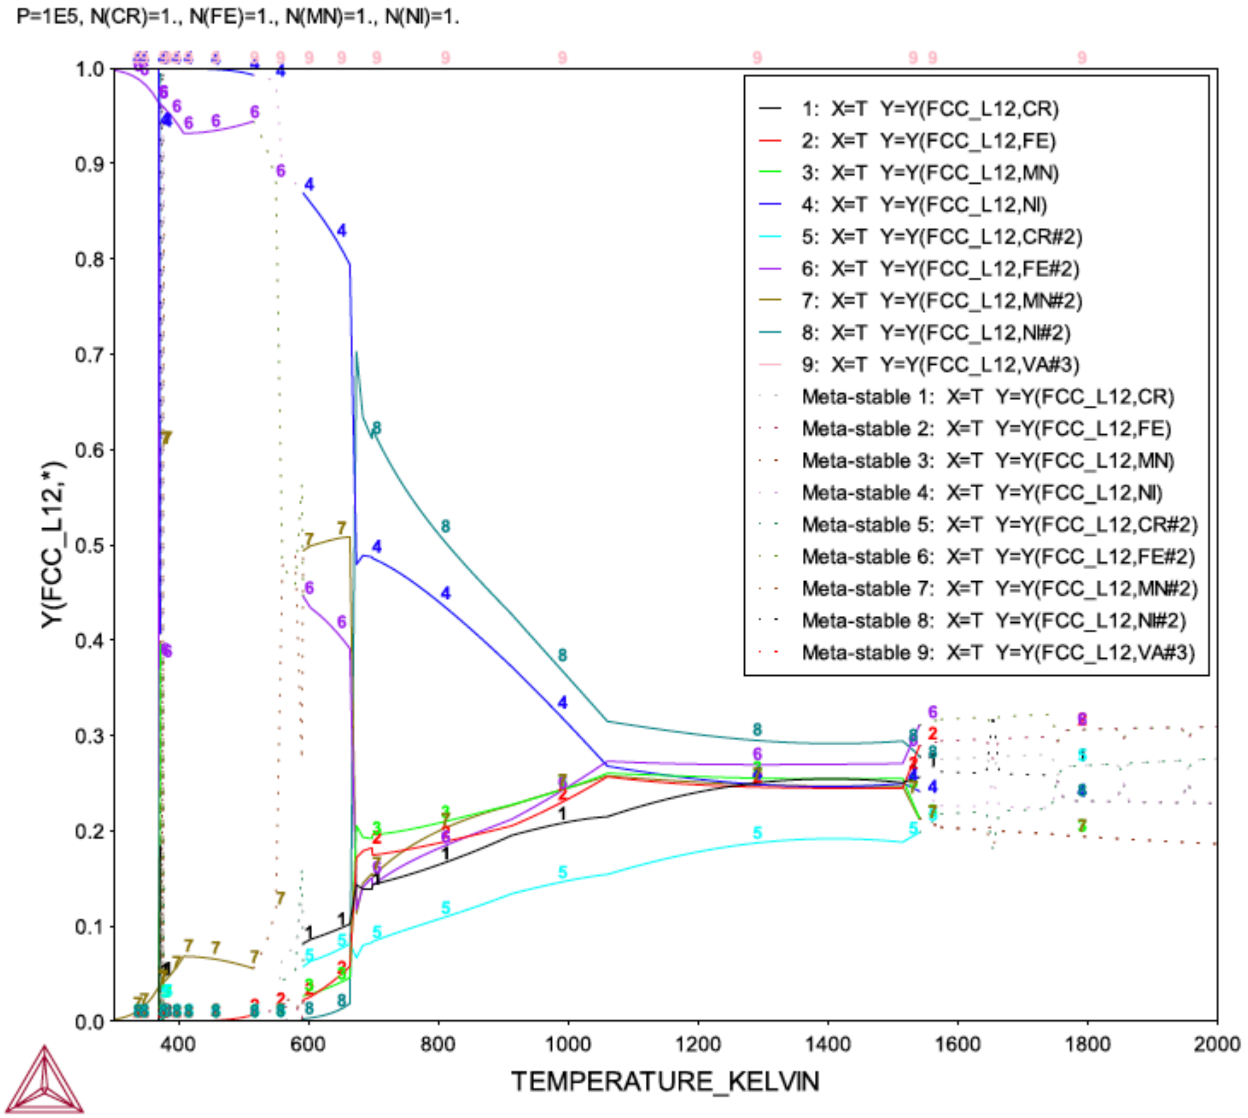


Figure F5. Site fraction calculations in the CrFeMnNi quaternary
